# Supplementary material for: LowRA: Accurate and Efficient LoRA Fine-Tuning of LLMs under 2 Bits
Source: arXiv:2502.08141 source file (2025-02-12)
Supplement: Supplementary file 1 [file mapping_only.tex]

\section{Searching Mappings for Different Downstream Tasks With Task-agnostic Base Weight} \label{app:stemappingsearch}

In many scenarios, we fix a \emph{task-agnostic} set of bin boundaries (thresholds) when quantizing base model weights---e.g., learned or derived from an offline procedure independent of specific tasks. 
However, each downstream task can have its own \emph{task loss}, which may not be purely mean-squared error (MSE). For instance, the task might involve classification with cross-entropy loss, or language modeling with a negative log-likelihood objective. 
In such cases, one can \emph{fine-tune} the \emph{mappings} (\emph{codepoints}) of the quantizer to minimize the specific downstream task loss while keeping the thresholds fixed.

\paragraph{Setup.} Let 
\(
  \theta_0 = -\infty < \theta_1 < \cdots < \theta_{B-1} < \theta_B = +\infty
\)
be the fixed thresholds. We partition real values into \(B\) bins, and each bin \(j\) has a representative codepoint \(m_j\). 
Any weight \(x_i\) is quantized to
\[
   Q(x_i) \;=\; m_{\mathrm{bin}(x_i)},
   \qquad
   \mathrm{bin}(x_i) = j 
   \;\;\Longleftrightarrow\;\;
   \theta_{j-1} < x_i \le \theta_j.
\]

\paragraph{Task Loss.} 
Unlike a purely reconstruction-based objective (e.g., MSE), we consider a general \(\mathcal{L}\)-based downstream task loss, which depends on the \emph{quantized} weights. If the downstream model parameters are partly or fully replaced by \(\{Q(x_i)\}\), then the task loss for a given set of codepoints \(\{m_j\}\) can be written as
\[
   \mathcal{L}\bigl(\{m_j\}\bigr)
   \;=\; 
   \text{TaskLoss}\Bigl(\underbrace{Q(x_1), \,Q(x_2), \,\dots,\, Q(x_n)}_{\text{quantized parameters}}\Bigr).
\]
Examples include cross-entropy in classification tasks, negative log-likelihood in language modeling, or other differentiable objectives.

\paragraph{Optimization.} 
We now seek to minimize \(\mathcal{L}(\{m_j\})\) w.r.t.\ the codepoints \(\{m_j\}\), while the thresholds \(\{\theta_j\}\) remain fixed from a task-agnostic stage:
\[
   \min_{m_1, \dots, m_B} \quad \mathcal{L}\bigl(\{m_j\}\bigr).
\]
In practice, this can be done via gradient-based methods (e.g., Adam), by treating each \(m_j\) as a trainable parameter and backpropagating through the downstream task. 
During each gradient step,
\[
   \frac{\partial \mathcal{L}}{\partial m_j}
   \;=\;
   \sum_{i \,\in\, \mathcal{B}_j} \,
       \frac{\partial \mathcal{L}}{\partial Q(x_i)}
       \,\frac{\partial Q(x_i)}{\partial m_j}
   \;\;=\;\;
   \sum_{i \,\in\, \mathcal{B}_j} \,
       \frac{\partial \mathcal{L}}{\partial Q(x_i)},
   \quad
   \text{since }Q(x_i)=m_j \text{ for } x_i\in \mathcal{B}_j.
\]
(This expression assumes straight-through estimation for non-differentiable assignments; in many frameworks, one can approximate the binning operation with a gradient-through-identity trick.)

By fixing thresholds \(\{\theta_j\}\) from a generic or \emph{task-agnostic} quantizer, and only adjusting the mappings \(\{m_j\}\) to a \emph{task-specific} loss, we enable lightweight adaptation. Each downstream task simply refines the codepoints to optimize its own objective, while sharing the same partition of the real line. This approach balances the benefits of a universal bin structure with the flexibility of per-task mapping calibration.
